# Supplementary material for: Rethinking Performance Analysis for Configurable Software Systems: A Case Study from a Fitness Landscape Perspective
Source: arXiv:2412.16888 source file (2025-01-02)
Supplement: Supplementary file 1 [file additional.tex]

\begin{figure*}[t!]
    \centering
    \includegraphics[width=\linewidth]{figs/ASE_RQ2.pdf}
    \caption{Distribution of pairwise comparison results across different workloads of each system. Specifically: (A, B): the Pearson and Spearman correlation between fitness distribution, respectively. (C, D) The shake-up metric and Jaccard similarity between top $10\%$ regions. (E, F): The EMD and Jaccard similarity between the set of local optima configurations. (G, H): The Manhattan distance and rank shift between global optima configurations. (I, J): The Spearman correlation between option importance and interaction.}
    \label{fig:transfer}
\end{figure*}

\subsection{Configuration Landscape Across Workloads}

We conduct our analysis of landscape similarity at different levels of granularity that become increasingly stringent.

\noindent \textbf{\textit{F13.} Overall structural similarity. } We begin with a general comparison of the landscapes structural characteristics of each software system across different workloads. 

\ul{\textit{Significance.}} \, With overall structural similarity in of the landscapes across workloads of a same system, we can then expect similar optimizer behavior and model generalization. This could inform transfer learning in performance modeling, warm-starting of optimization, or the design of system-specific optimizers.

\ul{\textit{Methods.}} \, We first reviewed the landscape features discussed previously, with focus on the difference across workloads. We then assessed both linear and non-linear correlations in their fitness distributions using Pearson and Spearman correlation coefficients, respectively. We plot the distribution of pairwise correlation across all workloads in each system in \pref{fig:transfer}A and B.

\ul{\textit{Results.}} \, First, recap that most landscape features, e.g., the number of local optima, autocorrelation, and FFI, etc., in~\pref{fig:rq1},~\pref{fig:rq2_corr} and~\pref{fig:rq2} are highly consistent across different workloads of each system. These support the existence of structural similarity in these landscapes. The results in Figures~\ref{fig:transfer}A and B further confirmed this with clear correlation between fitness distributions. 

\noindent \textbf{\textit{F14.} Prominent regions.} While the previous analyses give a comprehensive comparison of structural similarity across the entire landscapes, here we zoom in to see whether the most prominent regions in the landscape are also shared across workloads.

\ul{\textit{Significance.}} \, Often one is more concerned with the most performant regions in the landscape, as they are the goal of the optimization. If such regions are shared across workloads, we can then start the search directly from them~\cite{PoloczekWF16}, or leverage such knowledge to narrow down the search space~\cite{LustosaM24}, thereby speed up optimization.

\ul{\textit{Methods.}} \, We focused on the top $10\%$ configurations in each landscape. We measured the overlap between these regions across workloads using the \textit{Jaccard similarity}. In addition, we also considered another measure, namely the \textit{Shake-up score}, which is orginally developed to determine the shift in performance ranks of models in Kaggle competitions when the test data changes~\cite{RoelofsSRFHMS19}. Here we adapted it to evaluate the expected rank shift of the top $10\%$ configurations in one workload when evaluated in another workload, normalized by the total number of configurations. 

\ul{\textit{Results.}} \, We found that the overlap between the top $10\%$ regions of different workloads is typically small for our studied systems, as indicated by the Jaccard similarity in~\pref{fig:transfer}D. This implies that transferring prominent configurations may not yield directly comparable performance. Still, from the Shake-up metrics reported in~\pref{fig:transfer}C, we saw that for \textsc{Apache} and \texttt{SQLite}, the expected rank shift is very small, with an average of $3.9\%$ and $6.1\%$, respectively. However, significant rank shifts were observed for \textsc{LLVM} ($34.92\% \pm 26.7\%$). While this result is somewhat counterintuitive, a possible reason for this is that the fitness values, i.e., running time, of \textsc{LLVM} are typically at a small scale (e.g., $<1$ for several workloads), and the difference between top configurations are narrow. This then renders fitness ranks very sensitive to subtle changes in values. Despite this, in practice, when we are more interested in the values of the run time (rather than ranks), the transferred top configurations may still be able to offer competitive performance.

\noindent \textbf{\textit{F15.} Local optima. } Given the similarity in global landscape topographies across workloads, it is then intriguing to investigate whether the sets of local optima, are also shared across them. This includes $i-ii)$ the number and configurations of local optima, and $iii)$ their distributions.

\ul{\textit{Significance.}} \, Since local optima are one of the main obstacles in optimization, similar information regarding them across workloads of a same system can be exploited to design bespoke solvers~\cite{Prugel-BennettT12} to avoid them. On the other hand, considering the fact that local optima can often outperform random configurations in the landscape (\pref{fig:rq1} (E)), it is also a good idea to reuse them across workloads.

\ul{\textit{Methods.}} \, We explored the $4$ aspects outlined above one by one. We have previously measured the number of local optima in each workload as in~\pref{fig:rq1} (A). We then calculated the overlap between the sets of local optima configurations in different workloads using the \textit{Jaccard similarity}. Yet, this is a rather strict criterion as it seeks exact matches between configurations. Alternatively, we hypothesize that the local optima in different workloads distribute similarly in the landscape, but undergo slight ``shifts''. To quantify the such distributional similarity of local optima, we used the \textit{Earth Mover's Distance (EMD)}~\cite{RubnerTG00} from the classic optimal transport framework. It quantifies the minimal ``work'' (i.e., distance) required to relocate a set of local optima in a landscape into a different distribution (as in a different landscape). 

\ul{\textit{Results.}} \, We found that the local optima are rarely shared across workloads for all $3$ studied systems, as indicated by the low Jaccard similarity (on average $2.16\%$ across all $32$ landscapes). Albeit this, it is intriguing to see that the distribution of local optima in different workloads exhibit close proximity. For example, the average EMD between the set of local optima in \textsc{LLVM} workloads is $2.69 \pm 0.38$, which is quite low compared to the diameter of the landscape, i.e., $20.0$.

\noindent \textbf{\textit{F16.} Global optimum. } Among all local optima, of particular interest is the global optimum. Here, given two workloads $W_a$ and $W_b$ of a system and their global optima $\mathbf{c}^{*(a)}$ and $\mathbf{c}^{*(b)}$, we explore two aspects: $i)$ the distance $d(\mathbf{c}^{*(a)}, \mathbf{c}^{*(b)})$, $ii)$ the rank shift $|R_a(f_a(\mathbf{c}^{*(a)})) - R_b(f_b(\mathbf{c}^{*(a)}))|$, and likewise, $|R_a(f_a(\mathbf{c}^{*(b)})) - R_b(f_b(\mathbf{c}^{*(b)}))|$.

\ul{\textit{Significance.}} \, If the global optimal configurations of different workloads lie closely in the landscape with robust performance, then we may directly reuse the same configuration.

\ul{\textit{Methods.}} \, We measured the distances and rank shifts as described above between global optima of each pair of workloads of a system. We report the results in \pref{fig:transfer}?.

\ul{\textit{Results.}} \, We observed considerable difference in the global optimal configurations in different workloads. For example, the average pairwise Manhattan distance for \textsc{Apache} is $11.75 \pm 3.82$, comparable to the radius ($9.0$) of the landscape. Fortunately, we then saw from \pref{fig:transfer}?? that the shift in performance rank when transferring the global optimum configuration from one workload of \textsc{Apache} to another is very small, with an average of $0.44\% \pm 0.08\%$. This is also true for \texttt{SQLite}, where the average rank shift is only $0.1\% \pm 0.03\%$. However, again, rank shifts for transferring global optimum between workloads of \textsc{LLVM} are significant ($40.01\% \pm 13.9\%$). 

\noindent \textbf{\textit{F17.}Feature importance and interaction.} We finalize our analysis by investigating the consistency of measured option importance and interaction across workloads.

\ul{\textit{Significance.}} \, Previous works assume that feature importance and their interactions are transferable across workloads~\cite{JamshidiSVKPA17}. We wonder whether this assumption holds true for all workloads and systems. If it does not, it is necessary to consider the potential distortion of feature importance and interactions when transferring across different workloads. 

\ul{\textit{Methods.}} \, We had previously quantified the influence of each individual option in \textit{\textbf{F10}} and their interactions in \textit{\textbf{F12}}. Here, we used the Spearman correlation coefficient to assess the consistency of option importance and interaction across workloads. These results are shown in~\pref{fig:transfer}I and J. 

\ul{\textit{Results.}} \, From the results, we could see that for all $3$ systems, in general, both option importance and interaction are preserved across workloads, yet in several cases where the workload difference is significant, there could be strong distortion in option importance and interaction. For example, in the \textsc{LLVM} system, some workloads exhibit weak correlation ($\leq$0.1), indicating significant variability in feature interactions, while \textsc{APACHE} and \textsc{SQLITE} exhibit higher median correlations.

\clearpage

\begin{figure}[t!]
    \centering
    \includegraphics[width=\linewidth]{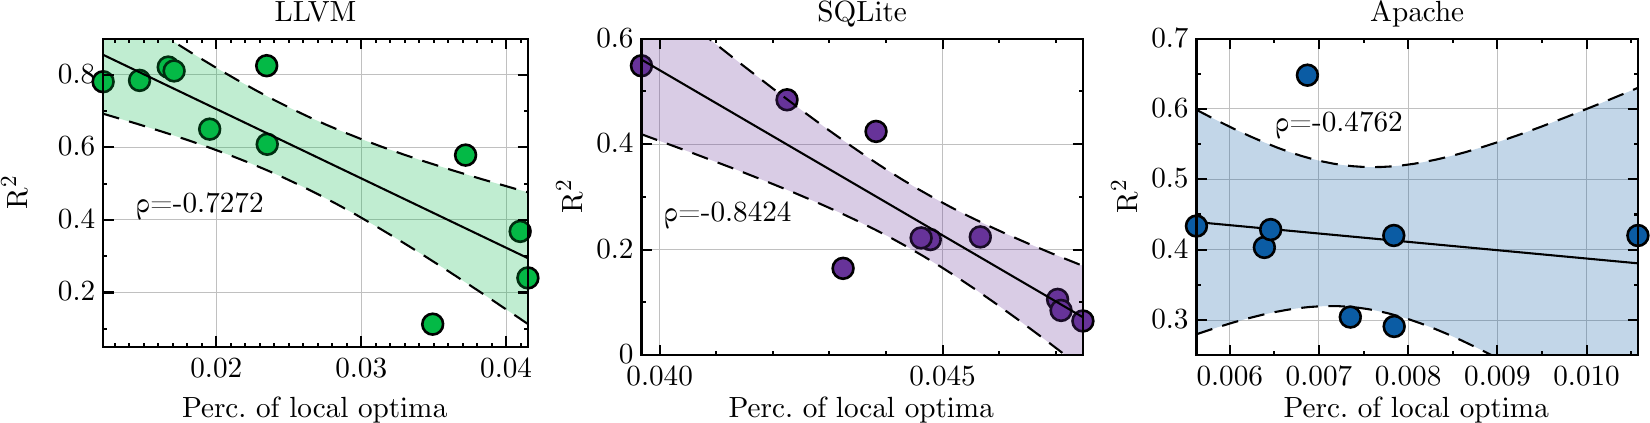}
    \caption{The predictability of the configuration landscapes as measured by $\mathrm{R^2}$ score of a XGBoost regressor on the hold-out test set decreases with the increase of landscape ruggedness across all $3$ systems. Linear regressions lines, with $95\%$ confidence intervals and Spearman correlation are also displayed.}
    \label{fig:predictability}
\end{figure}

\section{Landscape Modeling}

\noindent \textbf{\textit{F17.} Landscape predictability.} 

\ul{\textit{Results.}} \, Intruigingly, we found that both the percentage of local optima and the autocorrelation are highly correlated with the predictability of the configuration landscapes, despite a relatively weaker strength on \textsc{Apache} (\pref{fig:predictability}). The effects of such correlation is remarkably pronounced. For example, for \textsc{LLVM}, the $\mathrm{R^2}$ coefficient of the XGBoost on the test set can drop from $0.825$ (\texttt{syr2k}) to $0.113$ (\texttt{deriche}) when encountering a $\approx50\%$ ($24,620 \to 36,633$) increase in the number of local optima. Similar trends can also be observed when considering other performance models (Appendix \textbf{??}). 

Previous clues have hinted at such relationship between landscape ruggedness and predictability. For example, \dots. 

Also, in machine-guided protein engineering~\cite{YangWA19}, the local fitness landscape of a green fluorescent protein~\cite{Sarkisyan16}, which has a rather rugged surface, presents a challenging benchmark task for predictive models (see Table 2 of~\cite{RaoBTDCCAS19}). In constrast, prediction on more benign landscapes can be much easier.

It is also in concordance with simulations on $NK$ landscapes with varying dimensions, for which landscape predictability are found to progressively decrease with the increase of the ruggedness parameter $k$ (Appendix \textbf{??}). 

\clearpage
