# Supplementary material for: Rethinking Performance Analysis for Configurable Software Systems: A Case Study from a Fitness Landscape Perspective
Source: arXiv:2412.16888 source file (2025-01-02)
Supplement: Supplementary file 2 [file appendix.tex]

\section{Workloads and Configuration Options}

We provide the full list of selected configuration options used in our case study for the three subject systems: \textsc{LLVM} (\pref{tab:llvm_parameters}), \textsc{SQLite} (\pref{tab:sqlite_parameters}), and \textsc{Apache} (\pref{tab:apache_parameters}). We also provide the full list of workloads used in our case study for the three subject systems in \pref{tab:environment_lookup}.

\begin{table}[h!]
    \centering
    \small
    \caption{Selected configuration options for \textsc{LLVM}}
    \label{tab:llvm_parameters}
    \begin{tabular}{||ccc||}
        \hline
        Index & Parameter & Value \\ \hline \hline
        $1$ & \texttt{inline} &$\{\texttt{on},\texttt{off}\}$ \\
        $2$ & \texttt{openmpopt} & $\{\texttt{on},\texttt{off}\}$ \\
        $3$ & \texttt{mldst-motion} & $\{\texttt{on},\texttt{off}\}$ \\
        $4$ & \texttt{gvn} &$\{\texttt{on},\texttt{off}\}$ \\
        $5$ & \texttt{jump-threading} &$\{\texttt{on},\texttt{off}\}$ \\
        $6$ & \texttt{correlated-propagation} &$\{\texttt{on},\texttt{off}\}$ \\
        $7$ & \texttt{elim-avail-extern} &$\{\texttt{on},\texttt{off}\}$ \\
        $8$ & \texttt{tailcallelim} &$\{\texttt{on},\texttt{off}\}$ \\
        $9$ & \texttt{constmerge} &$\{\texttt{on},\texttt{off}\}$ \\
        $10$ & \texttt{dse} &$\{\texttt{on},\texttt{off}\}$ \\
        $11$ & \texttt{slp-vectorizer} &$\{\texttt{on},\texttt{off}\}$ \\
        $12$ & \texttt{callsite-splitting} &$\{\texttt{on},\texttt{off}\}$ \\
        $13$ & \texttt{argpromotion} &$\{\texttt{on},\texttt{off}\}$ \\
        $14$ & \texttt{aggressive-instcombine} &$\{\texttt{on},\texttt{off}\}$ \\
        $15$ & \texttt{polly-simplify} &$\{\texttt{on},\texttt{off}\}$ \\
        $16$ & \texttt{polly-dce} &$\{\texttt{on},\texttt{off}\}$ \\
        $17$ & \texttt{polly-optree} &$\{\texttt{on},\texttt{off}\}$ \\
        $18$ & \texttt{polly-delicm} &$\{\texttt{on},\texttt{off}\}$ \\
        $19$ & \texttt{polly-opt-isl} &$\{\texttt{on},\texttt{off}\}$ \\
        $20$ & \texttt{polly-prune-unprofitable} &$\{\texttt{on},\texttt{off}\}$ \\ \hline
    \end{tabular}
  \end{table}

  \begin{table}[h!]
    \centering
    \small
    \caption{Selected configuration options for \textsc{Apache}}
    \label{tab:apache_parameters}
    \begin{tabular}{||ccc||}
        \hline
        Index & Parameter & Value \\ \hline \hline
        $1$ & \texttt{AcceptFilter} & $\{\texttt{nntp},\texttt{http}\}$ \\
        $2$ & \texttt{KeepAlive} & $\{\texttt{on},\texttt{off}\}$ \\
        $3$ & \texttt{KeepAliveTimeout} & $\{1,\ldots,300\}$ \\
        $4$ & \texttt{MaxKeepAliveRequests} & $\{1,\ldots,2^{10}\}$ \\
        $5$ & \texttt{TimeOut} & $\{1,\ldots,300\}$ \\
        $6$ & \texttt{MaxConnectionsPerChild} & $\{1,\ldots,1,000\}$ \\
        $7$ & \texttt{MaxMemFree} & $\{2^{10},\ldots,2^{20}\}$ \\
        $8$ & \texttt{MaxRequestWorkers} & $\{100,\ldots,3,000\}$ \\
        $9$ & \texttt{MaxSpareThreads} & $\{50,\ldots,500\}$ \\
        $10$ & \texttt{MinSpareThreads} & $\{20,\ldots,250\}$ \\
        $11$ & \texttt{SendBufferSize} & $\{2^{10},\ldots,2^{16}\}$ \\
        $12$ & \texttt{ServerLimit} & $\{100,\ldots,3,000\}$ \\
        $13$ & \texttt{StartServers} & $\{1,\ldots,10\}$ \\
        $14$ & \texttt{ThreadLimit} & $\{10,\ldots,200\}$ \\
        $15$ & \texttt{ThreadsPerChild} & $\{10,\ldots,200\}$ \\ \hline
    \end{tabular}
    \end{table}

  \begin{table}[h!]
    \centering
    \tiny
    \small
    \caption{Selected configuration options for \textsc{SQLite}}
    \label{tab:sqlite_parameters}
    \begin{tabular}{||ccc||}
        \hline
        Index & Parameter & Value \\ \hline \hline
        $1$ & \texttt{SQLITE\_SECURE\_DELETE} & $\{\texttt{on},\texttt{off}\}$ \\
        $2$ & \texttt{SQLITE\_TEMP\_STORE} & $\{0,1,2,3\}$ \\
        $3$ & \texttt{SQLITE\_ENABLE\_AUTO\_WRITE} &$\{\texttt{on},\texttt{off}\}$ \\
        $4$ & \texttt{SQLITE\_ENABLE\_STAT3} &$\{\texttt{on},\texttt{off}\}$ \\
        $5$ & \texttt{SQLITE\_DISABLE\_LFS} &$\{\texttt{on},\texttt{off}\}$ \\
        $6$ & \texttt{SQLITE\_OMIT\_AUTO\_INDEX} &$\{\texttt{on},\texttt{off}\}$ \\
        $7$ & \texttt{SQLITE\_OMIT\_BETWEEN\_OPT} &$\{\texttt{on},\texttt{off}\}$ \\
        $8$ & \texttt{SQLITE\_OMIT\_BTREECOUNT} &$\{\texttt{on},\texttt{off}\}$ \\
        $9$ & \texttt{SQLITE\_OMIT\_LIKE\_OPT} &$\{\texttt{on},\texttt{off}\}$ \\
        $10$ & \texttt{SQLITE\_OMIT\_LOOKASIDE} &$\{\texttt{on},\texttt{off}\}$ \\
        $11$ & \texttt{SQLITE\_OMIT\_OR\_OPT} &$\{\texttt{on},\texttt{off}\}$ \\
        $12$ & \texttt{SQLITE\_OMIT\_QUICKBALANCE} &$\{\texttt{on},\texttt{off}\}$ \\
        $13$ & \texttt{SQLITE\_OMIT\_SHARED\_CACHE} &$\{\texttt{on},\texttt{off}\}$ \\
        $14$ & \texttt{CacheSize} & $\{1,\ldots,10,240\}$ \\
        $15$ & \texttt{AutoVacuumON} & $\{0,1,2\}$ \\
        $16$ & \texttt{ExclusiveLock} &$\{\texttt{on},\texttt{off}\}$ \\
        $17$ & \texttt{PageSize} & $\{1,\ldots,10,240\}$ \\
        $18$ & \texttt{Wal} &$\{\texttt{on},\texttt{off}\}$ \\ \hline
    \end{tabular}
  \end{table}

  \begin{table*}[t!]
    \centering
    \small
    \caption{Lookup table of settings of different workloads for three configurable software systems.}
    \label{tab:environment_lookup}
    \begin{tabular}{||c|c|cccc}
        \hline
        $\mathcal{W}$ & \textsc{LLVM}             & \multicolumn{2}{c|}{\textsc{SQLite}}                                           & \multicolumn{2}{c||}{\textsc{Apache}}                                                        \\ \hline \hline
        \multicolumn{1}{||c|}{Index} & \texttt{program\_name} & \multicolumn{1}{c}{\texttt{num}} & \multicolumn{1}{c|}{\texttt{value\_size}} & \multicolumn{1}{c}{\texttt{requests}} & \multicolumn{1}{c||}{\texttt{concurrency}}  \\ \hline
        
        \multicolumn{1}{||c|}{$1$}     & 2mm              & \multicolumn{1}{c}{$10$}             & \multicolumn{1}{c|}{$100$}        & \multicolumn{1}{c}{$50$}                & \multicolumn{1}{c||}{$50$}                      \\ 
        \multicolumn{1}{||c|}{$2$}     & 3mm              & \multicolumn{1}{c}{$10$}             & \multicolumn{1}{c|}{$1,000$}       & \multicolumn{1}{c}{$100$}               & \multicolumn{1}{c||}{$100$}                     \\ 
        \multicolumn{1}{||c|}{$3$}     & atax             & \multicolumn{1}{c}{$10$}             & \multicolumn{1}{c|}{$10,000$}      & \multicolumn{1}{c}{$100$}               & \multicolumn{1}{c||}{$100$}                 \\ 
        \multicolumn{1}{||c|}{$4$}     & correlation      & \multicolumn{1}{c}{$10$}             & \multicolumn{1}{c|}{$30,000$}      & \multicolumn{1}{c}{$200$}               & \multicolumn{1}{c||}{$200$}                   \\ 
        \multicolumn{1}{||c|}{$5$}     & covariance       & \multicolumn{1}{c}{$100$}            & \multicolumn{1}{c|}{$100$}        & \multicolumn{1}{c}{$250$}               & \multicolumn{1}{c||}{$250$}                 \\ 
        \multicolumn{1}{||c|}{$6$}     & deriche          & \multicolumn{1}{c}{$100$}            & \multicolumn{1}{c|}{$100$}        & \multicolumn{1}{c}{$300$}               & \multicolumn{1}{c||}{$300$}               \\ 
        \multicolumn{1}{||c|}{$7$}     & doitgen          & \multicolumn{1}{c}{$100$}            & \multicolumn{1}{c|}{$1,000$}       & \multicolumn{1}{c}{$400$}               & \multicolumn{1}{c||}{$400$}                    \\ 
        \multicolumn{1}{||c|}{$8$}     & fdtd2d           & \multicolumn{1}{c}{$100$}            & \multicolumn{1}{c|}{$10,000$}      & \multicolumn{1}{c}{$500$}               & \multicolumn{1}{c||}{$500$}                    \\ 
        \multicolumn{1}{||c|}{$9$}     & gemm             & \multicolumn{1}{c}{$100$}            & \multicolumn{1}{c|}{$30,000$}      & \multicolumn{1}{c}{$1,000$}              & \multicolumn{1}{c||}{$100$}                \\ \cline{5-6}
        \multicolumn{1}{||c|}{$10$}    & symm             & \multicolumn{1}{c}{$1,000$}           & \multicolumn{1}{c|}{$10$}         &                                                              \\ \cline{3-4} 
        \multicolumn{1}{||c|}{$11$}    & syr2k            &                                     &                                 &                                        &                                                                   \\ 
        \multicolumn{1}{||c|}{$12$}    & syrk             &                                     &                                 &                                        &                                                   \\ 
        \multicolumn{1}{||c|}{$13$}    & trmm             &                                     &                                 &                                        &                                                   \\ \cline{1-2}  
    \end{tabular}
\end{table*}
